# Supplementary material for: NPMs: Neural Parametric Models for 3D Deformable Shapes
Source: arXiv:2104.00702 source file (2021-08-05)

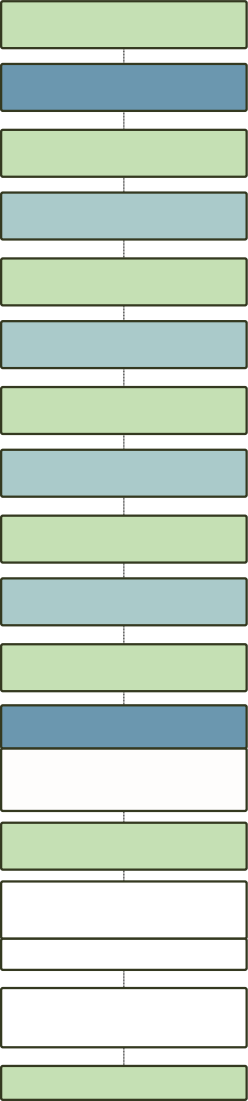

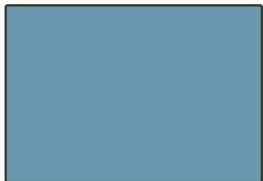

|  |
|--|
|  |
|  |
|  |

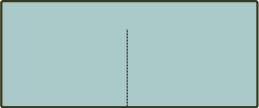

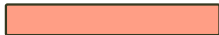

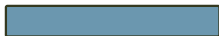

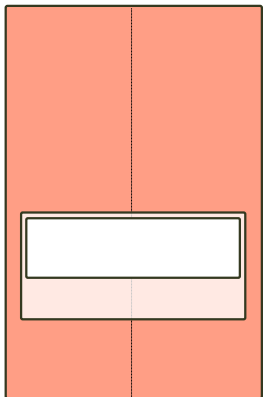



|  |
|--|
|  |
|  |
|  |

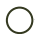

Supplement: Supplementary file 2 [file encoder.pdf]
