# Supplementary material for: NPMs: Neural Parametric Models for 3D Deformable Shapes
Source: arXiv:2104.00702 source file (2021-08-05)

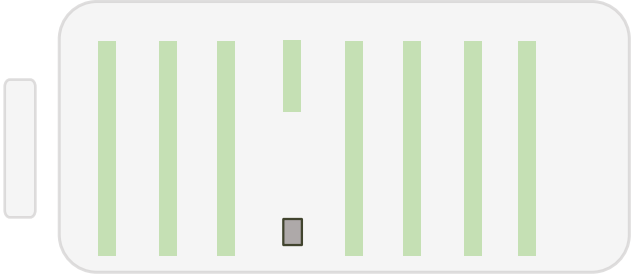

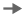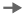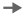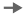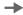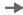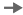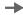

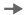

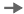

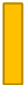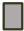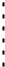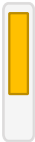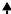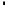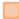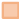

Supplement: Supplementary file 4 [file shape_mlp_detail.pdf]
